# Supplementary material for: Controlling a quantum point junction on the surface of an antiferromagnetic topological insulator
Source: arXiv:2008.03316 ancillary file (2020-08-07)
Supplement: Supplementary file 1 [file supplemental_info.pdf]

# Supplementary Information
# Controlling a quantum point junction on the surface of an antiferromagnetic topological insulator


Nicodemos Varnava,* Justin H. Wilson, J. H. Pixley, and David Vanderbilt
*Department of Physics & Astronomy, Center for Materials Theory, Rutgers University, Piscataway, New Jersey 08854, USA*


## I. BULK AND SURFACE STATES

For completeness we repeat the bulk Hamiltonian

$$H_0 = m\sum_{\ell} c_{\ell}^{\dagger}\tau^{z}c_{\ell} + +m_{\rm Z}\sum_{\ell}(-)^{\ell_z}c_{\ell}^{\dagger}\sigma^{z}c_{\ell} + \frac{t}{2}{\sum_{\ell\ell'}}' c_{\ell}^{\dagger}\tau^{z}c_{\ell'} + \frac{-i\lambda}{2}{\sum_{\ell\ell'}}' c_{\ell}^{\dagger}\tau^{x}\hat{\mathbf{n}}_{\ell\ell'}\cdot\boldsymbol{\sigma}c_{\ell'}\ . \quad \text{(S1)}$$

From left to right, the four terms describe the onsite energies, staggered Zeeman field, and spin-independent and spin-depended nearest-neighbor hoppings. We first consider the case where $m_Z = 0$, in which case the Hamiltonian $H_0$ reduces to the time-reversal ($\mathcal{T}$) symmetric model proposed by Bernevig et al.[S1,S2] $\mathcal{T}$ symmetry is an axion-odd symmetry, meaning the axion coupling is quantized to $\theta = 0$ or $\pi$ in its presence. At half-filling and for $(m, t, \lambda) = (1.0, -0.5, -0.6)$, the ground state has $\theta = \pi$, corresponding to a strong topological insulator (STI). The bulk-boundary correspondence then implies the presence of $\mathcal{T}$-protected surface Dirac cones, as illustrated in Fig. **S1c** for the (001) surface.

For $m_Z = -0.3$, even though $\mathcal{T}$ is broken, $\mathcal{T}$ followed by a half-lattice translation along $\hat{\mathbf{z}}$ ($\mathcal{T} * \tau_{1/2}$) is a good symmetry. This symmetry is axion-odd as well[S3,S4] and $\theta = \pi$ for the above choice of parameters, making it an AFM-TI insulator. An important difference between $\mathcal{T}$ and $\mathcal{T} * \tau_{1/2}$ is that the latter symmetry does not force the surface AHC of all surfaces to vanish. In fact, Fig. **S1f** shows that the AFM Zeeman term opens the (001) surface gap, with the top and bottom surfaces exhibiting a half-integer $(n + 1/2)e^2/h$ AHC, where $n$ depends on the surface termination.[S5]

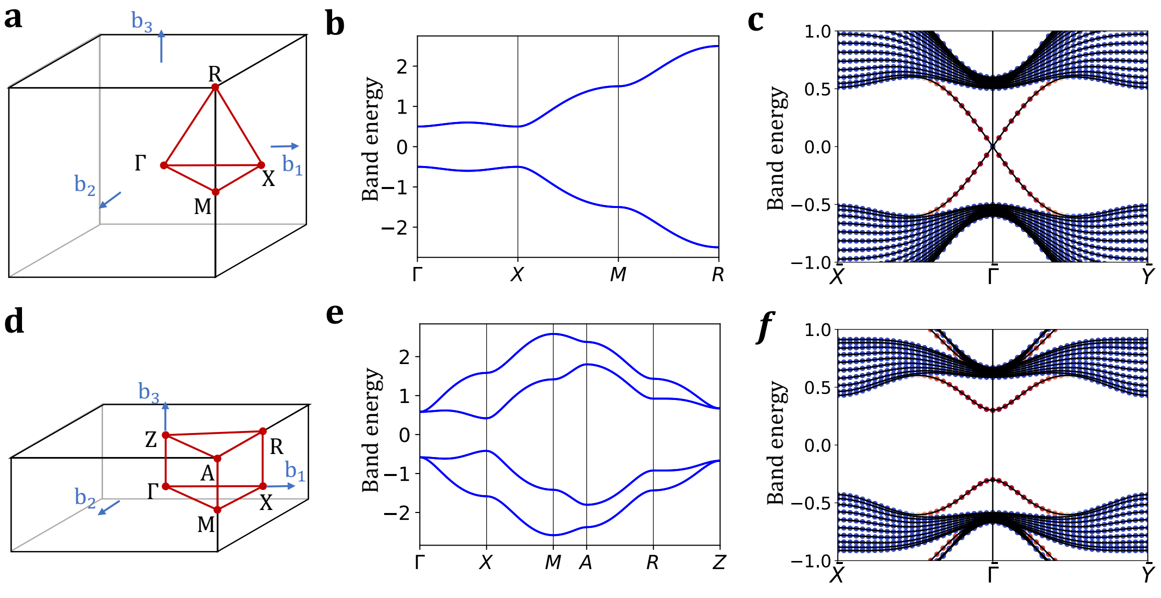


FIG. S1. **a**, Brillouin zone, **b**, bulk bands and **c**, surface bands along (001) for the STI model. **d-f** Same for the AFM-TI model. In **b**, **e**, the bands are doubly degenerated due to time-reversal composed with inversion $\mathcal{T} * \mathcal{I}$ and in **c**, **f**, red/blue markers indicate surface/bulk bands.

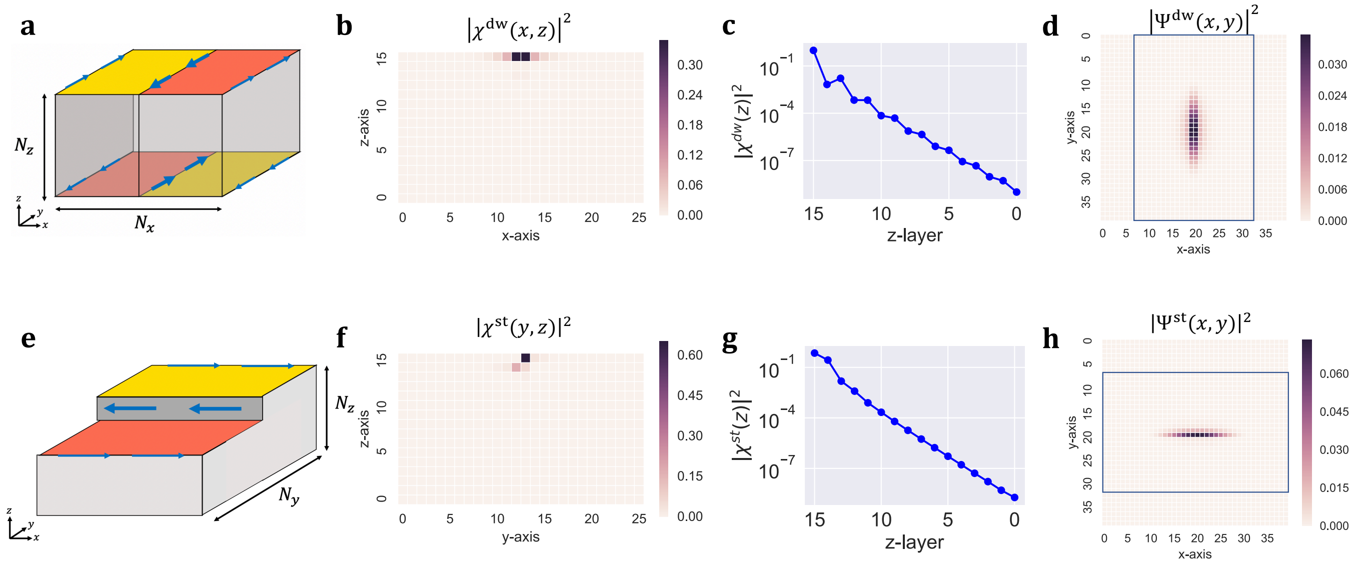


FIG. S2. **a**, Sketch of the AFM-TI supercell slab with a domain-wall in direction $y$ and the associated energy states. **b**, Spatial profile of the transverse shape of the WP $|\chi^{\rm dw}(x,z)|^2 = \sum_{\sigma\tau} |\chi^{\rm dw}_{\sigma\tau}(x,z)|^2$. **c**, Logarithmic plot of the layer density $|\chi^{\rm dw}(z)|^2 = \sum_x |\chi^{\rm dw}(x,z)|^2$ which shows the exponential localization of the states at the surface. **d**, The initial (001)-projected domain-wall WP $|\Psi^{\rm dw}(x,y)|^2 = \sum_{\sigma\tau,z} |\Psi^{\rm dw}_{\sigma\tau}(x,y,z)|^2$. Note that the constructed WP (inside the box) has been placed in a larger system with zero amplitude assigned outside the box. **e-h**, Same as **a-d**, but for a step along the $x$ direction. Comparing **b** and **f**, we see that in the case of a step the surface state wavefunction redistributes itself across the two surfaces in an unequal manner.

## II. WAVE PACKET CONSTRUCTION

For clarity we focus on the construction of domain-wall channel WPs, since the construction of step channel WPs follows in a similar fashion. We start by considering an $N_x \times 1 \times 1$ supercell of the AFM-TI model and use it to create a slab that is $N_z$ unit cells thick along (001). Because of the periodic boundary conditions, we have no choice but to create two domain walls. We choose these to be centered at the $x = 1/2$ and $(N_x + 1)/2$ planes, and create them by flipping the Zeeman potential of all orbitals in the half-cell to the left of the $x = 1/2$ plane. We refer to the Hamiltonian of this slab supercell with a pair of domain walls as $\hat{H}_{\rm dw}$. Fig. S2**a** shows a sketch of the slab supercell while the associated energy bands were presented in the main text Fig. **1c** for a supercell with $N_x = 20$ and $N_z = 8$. We see that two counter-propagating, doubly degenerate, linear bands appear in the insulating gap, corresponding to the four chiral channels indicated with blue arrows in Fig. S2**a** (note the in-plane periodic boundary conditions).

The Bloch eigenvectors of $\hat{H}_{\rm dw}$ are $\psi^{\rm dw}_{nk_y\sigma\tau}(\mathbf{r}) = e^{ik_y y}\, u^{\rm dw}_{nk_y\sigma\tau}(x,z)$, where $u^{\rm dw}_{nk_y\sigma\tau}$ are the cell-periodic counterparts. Note that we neglect the exponentially small dispersion along the $k_x$-direction, and the $y$ dependence is absent from $u^{\rm dw}_{nk_y\sigma\tau}$ because there is only a single site per unit cell. A technical difficulty arises from the fact that the chiral channels are doubly degenerate as a result of the $I * T$ symmetry of $\hat{H}_{\rm dw}$, but we extract channel-localized states by diagonalizing the $z$ operator in the space of the two degenerate states. We denote the channel-localized states as $\tilde{u}^{\rm dw}_{\nu k_y\sigma\tau}(x,z)$, where the index $\nu$ labels the four chiral channels.

The final step in constructing our initial WPs is to take quantum superpositions of channel-localized Bloch states $\tilde{\psi}^{\rm dw}_{\nu k_y\sigma\tau}(\mathbf{r})$ according to a Gaussian envelope function $F(k_y) = A\exp\left(-k_y^2/2\kappa^2\right)$ centered at $k_y = 0$, where $A$ is a normalization factor and $\kappa$ is a measure of the extent of the WP along the channel.[S6] Our initial WPs for the domain-wall are then

$$\Psi^{\rm dw}_{\sigma\tau}(\mathbf{r}, t=0) \;=\; \int_{-\pi}^{\pi} dk_y\, F(k_y)\, \tilde{\psi}^{\rm dw}_{\nu k_y\sigma\tau}(\mathbf{r}). \tag{S2}$$

At this point we make the additional approximation $\tilde{u}^{\rm dw}_{\nu k_y\sigma\tau}(x,z) = \tilde{u}^{\rm dw}_{\nu 0\sigma\tau}(x,z)$, which is well justified for a WP of sufficiently narrow extent in $k_y$. We note that this approximation is equivalent to the WP decomposition of Eq. (1) in the main text with the identification

$$\chi^{\rm dw}_{\sigma\tau}(x,z) = \tilde{u}^{\rm dw}_{\nu 0\sigma\tau}(x,z), \qquad f(r) = \int_{-\pi}^{\pi} dk\, e^{ikr} F(k). \tag{S3}$$

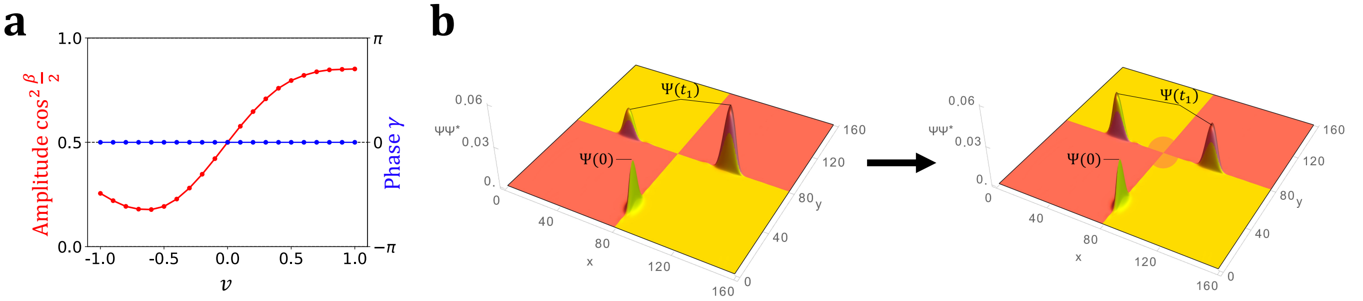


FIG. S3. **a**, Magnitude $\cos^2(\beta/2)$ and phase $\gamma$ (defined in Eq. (7) of the main text) as a function the strength of the mirror breaking hopping term $v$ . Only the magnitude is modified by the addition of this term. **b**, Setting $v = 0.24$ in Eq. (S4) causes unequal splitting of the WP but we can use the magnetic tip with $V_Z = 0.14$ to cancel the effect of the mirror breaking term.

The WP construction for the case of the step channel follows in a similar way. Because the steps only need to be created at the top surface of the slab, the channel-localized states are nondegenerate. We note that the periodic boundary conditions enforce a second step channel, which produces states of both chirality in the dispersion shown in Fig. 1**d** of the main text. the The rest of the above discussion applies, but with $x \leftrightarrow y$ and $k_x \leftrightarrow k_y$ because we take the steps to propagate along $\hat{x}$.

## III. BREAKING SYMMETRIES

As discussed in the main text, the fact that the QPJ "naturally" implements the Hadamard gate is a manifestation of the high symmetry of the model and of the geometry of the junction. In this section we show how breaking the extraneous $M_x$ and $M_y$ mirror symmetries affects the S-matrix. To break these symmetries we add a mirror-breaking hopping term

$$V_M = \frac{-iv}{2} {\sum_{\ell\ell'}}' c_\ell^\dagger \tau^x \sigma^z c_{\ell'} \delta_{\ell_z \ell'_z} \ , \tag{S4}$$

where $\delta_{\ell_z \ell'_z}$ ensures that only in-plane hopping terms are considered. Note that this term couples spin and orbit in a way that preserves $\mathcal{T}$ symmetry.[S7] Even though Eq. (S4) does not affect the magnetic properties of the junction it nonetheless affects the S-matrix by modifying the magnitude splitting $\cos^2(\beta/2)$, as the numerical calculations indicate in Fig. **S3a**. Importantly, the universal control over the S-matrix magnitudes using the local magnetic tip enables us to eliminate (i.e., calibrate) the effect of the mirror-breaking terms, as illustrated in Fig. **S3b**.

## IV. STABILITY TO DISORDER

Finally we show that the QPJ is robust in the presence of disorder. We introduce disorder into the model Hamiltonian by adding a random potential scattering term given by

$$V_D = \sum_\ell m_D(\ell) c_\ell^\dagger c_\ell \ . \tag{S5}$$

The disorder potential $m_D(\ell)$ is sampled from a Gaussian distribution at each site in the three-dimensional lattice $\ell$ with zero mean and standard deviation $W$, which characterizes the strength of the disorder potential. For sufficiently large $W$ the average band gap in the bulk will close and the model will transition out of a topological phase. In contrast, for weaker disorder strengths (relative to the clean band gap, which is equal to $E_g \approx 0.6$ here) the topological properties are expected to remain robust. This should also provide a level of protection of the chiral surface states from back-scattering due to the disorder potential, but how this impacts the quantum point junction remains unclear.

To demonstrate the robustness of the junction to disorder, we have performed a similar analysis as in the previous section. In contrast with Sec. III, we cannot construct the initial WP from the exact eigenstates because of the presence of disorder in the system. For that reason, we use the same initial WP that was constructed for the clean model, and renormalize our results by accounting for the prompt loss of amplitude associated with the fact that this

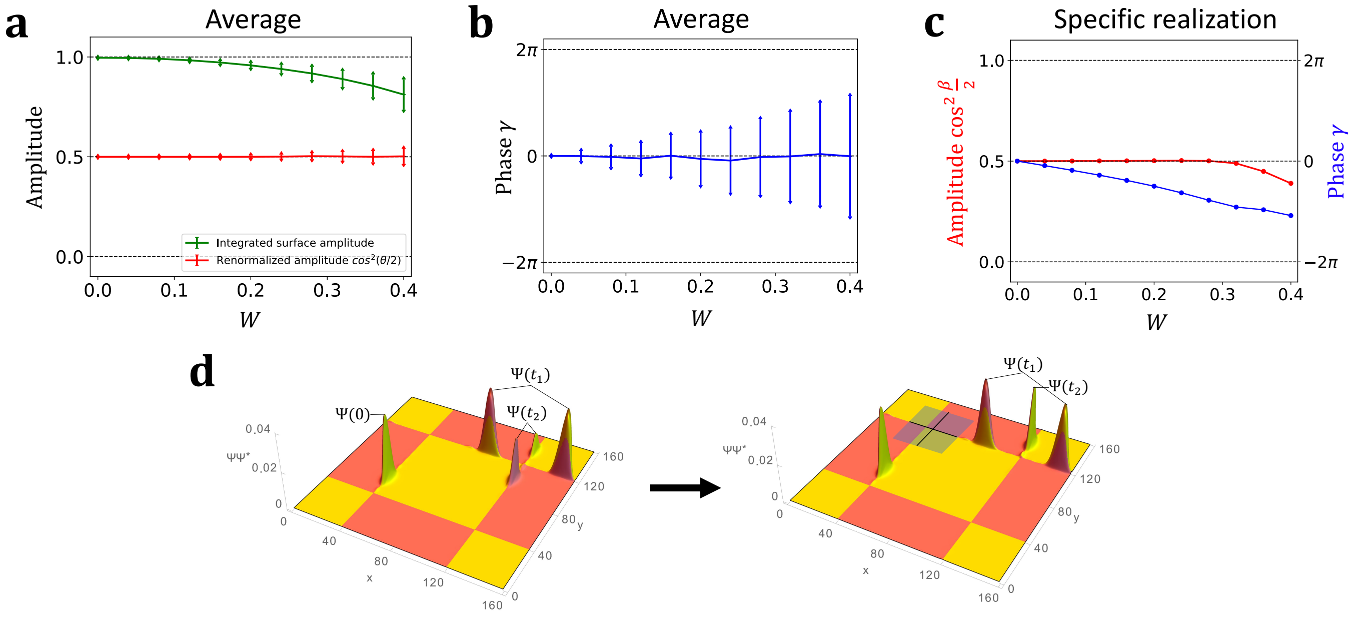


FIG. S4. **a**, **b**, Averaged magnitude splitting $\cos^2(\theta/2)$ and phase $\gamma$ over 20 disordered configurations for different values of $W$. **a**, Because the initial WP $\Psi(0)$ is not an exact eigenstate there is loss to the bulk we need to take into account. The green line shows the magnitude of the WP that remained on the surface after scattering at Junction 1 and the red line corresponds to the renormalized magnitude splitting. The disorder affects slightly the magnitude splitting which fluctuates about 50% for different realizations of disorder. **b**, The phase $\gamma$ is significantly affected by disorder and needs to be accounted. **c**, Example of a specific disorder realization as a function of $W$. **d**, For the realization in **c**, with $W = 0.1$ we can use the gate voltage tip to eliminate the random phase difference accumulated up to $t = t_2$, due to the disorder. In this example we set the strength of the gate voltage to $V_G = 0.1$ and the center of the rectangle at $(x_0, y_0) = (8, 0)$.

trial function has nonzero overlap with some extended bulk and surface states (see Fig. S4**a**). The results are averaged over 20 disorder samples and show that magnitude and phase evolution through the junction are randomly effected by disorder, and therefore retain the same average value as they do in the absence of disorder. In particular, the random potential induces both a splitting of the WP magnitude as well as a shift in the phase that are both random for each sample, which clearly averages to zero as demonstrated in Fig. **S4a**, **b**.

Lastly, we turn to how disorder can impact the QPJ in a specific disorder realization. We show that the effect of disorder can be calibrated adopting an approach like that used above for the mirror-breaking term. As shown in Fig. **S4c** for a specific random sample, the disorder does not affect the splitting, at least for small $W$, while the phase of the WP is significantly different from the clean limit. We then apply the gate voltage to completely remove this effect, returning the QPJ to its clean behavior, Fig. **S4d**. These results demonstrate both a robustness and a level of control over disorder in this novel QPJ. This is important, as each device made out of such a QPJ will have some random disorder profile. Nevertheless, as we have shown in Fig. **S4**, the electrostatic STM tip can be used to remove this effect, returning the QPJ to its ideal behavior.

---

* nvarnava@physics.rutgers.edu
[S1] B. A. Bernevig, T. L. Hughes, and S.-C. Zhang, Science **314**, 1757 (2006).
[S2] T. L. Hughes, E. Prodan, and B. A. Bernevig, Phys. Rev. B **83**, 245132 (2011).
[S3] R. S. K. Mong, A. M. Essin, and J. E. Moore, Phys. Rev. B **81**, 245209 (2010).
[S4] N. Varnava, I. Souza, and D. Vanderbilt, Phys. Rev. B **101**, 155130 (2020).
[S5] N. Varnava and D. Vanderbilt, Phys. Rev. B **98**, 245117 (2018).
[S6] Note that the shape of the WP does not influence our analysis, but in more realistic applications, minimal excitations such as Levitons[S8,S9] might be more desirable.
[S7] B. J. Wieder and B. A. Bernevig, The axion insulator as a pump of fragile topology (2018), arXiv:1810.02373.
[S8] L. S. Levitov, H. Lee, and G. B. Lesovik, Journal of Mathematical Physics **37**, 4845 (1996).
[S9] D. A. Ivanov, H. W. Lee, and L. S. Levitov, Phys. Rev. B **56**, 6839 (1997).
